# Supplementary material for: On Decidability of Time-bounded Reachability in CTMDPs
Source: arXiv:2006.05498 source file (2020-06-09)
Supplement: Supplementary file 1 [file appendix_skolem_ctmdp.tex]

% !TEX root = main.tex
\section{Reduction of Bounded Skolem Problem to Problem~\ref{prob:prob_switch}}
\label{sec:app:skolem_ctmdp}

In this section, we provide a reduction from the bounded continuous Skolem problem to checking
if the optimal strategy in a CTMDP requires a switch.

First, we show a technical result that there is no loss of generality in assuming $z_0 = 0$ in the Skolem problem.
We denote the answer of the bounded continuous Skolem problem by $\SP(\mathbf a, \mathbf z_0)$ with $\mathbf a$ and $\mathbf z_0$ being respectively 
the vectors of coefficients and of initial conditions:
\begin{equation*}
\mathbf a:=[a_{n-1},a_{n-2},\ldots,a_0]^T,\quad \mathbf z_0:= \left[z_0,\frac{dz_t}{dt}\Big|_{t=0},\ldots,\frac{d^{n-1}z_t}{dt^{n-1}}\Big|_{t=0}\right]^T.
\end{equation*}
The following proposition shows that we can assume $z_0 = 0$ without loss of generality.

\begin{proposition}
\label{app:prop:skolem-init-0}
For any $\mathbf a,\mathbf z_0\in \mathbb Q^n$, there are $\mathbf b,\mathbf y_0$ with rational entries and $\mathbf y_0(1) = 0$ such that
\begin{equation}
\label{eq:BS_zero}
\SP(\mathbf a, \mathbf z_0) = \SP(\mathbf b, \mathbf y_0).
\end{equation}
\end{proposition} 
\begin{proof}
The proof relies on constructing a linear ODE that has the unique solution $y_t = t z_t$ for all $t\in[0,B]$. It is obvious that $y_0 = 0$ and $y_t=0$ for some $0<t<B$ if and only if $z_t=0$ for the same $0<t<B$. Therefore, \eqref{eq:BS_zero} holds. We define $\mathbf b:= [b_{2n-1},b_{2n-2},\ldots,b_0]$ such that the following two polynomials are the same
\begin{equation*}
s^{2n}+b_{2n-1}s^{2n-1}+b_{2n-2}s^{2n-2}+\ldots+ b_1 s + b_0 = \left(s^{n}+a_{n-1}s^{n-1}+\ldots+ a_1 s + a_0\right)^2,\quad \forall s\in\mathbb R.
\end{equation*}
The vector $\mathbf y_0$ is also constructed as
\begin{equation*}
\mathbf y_0(1) = 0,\quad \mathbf y_0(k+1) = k \mathbf z_0(k)\quad \forall\,\, k\in\set{1,2,\ldots,2n-1},
\end{equation*}
with $\mathbf z_0(n+k) := -\sum_{i=0}^{n-1} a_i \mathbf z_0(i+k)$ for all $k\in\set{1,2,\ldots,n-1}$. The function $y_t = t z_t$ has the initial condition specified by $\mathbf y_0$. It only remains to show that this function satisfies the linear ODE
\begin{equation*}
\left(s^{2n}+b_{2n-1}s^{2n-1}+\ldots+ b_1 s + b_0\right) y_t = 0,
\end{equation*}
where $s$ is treated as the differentiation operator.
The left-had side of the above ODE can be written as
\begin{align*}
& t\left(s^{2n}+b_{2n-1}s^{2n-1}+\ldots+ b_1 s + b_0\right) z_t + 
\left(2ns^{2n-1}+(2n-1)b_{2n-1}s^{2n-2}+\ldots+ b_1\right) z_t\\
 & = t \left(s^{n}+a_{n-1}s^{n-1}+\ldots+ a_1 s + a_0\right)^2 z_t \\
 & + 2 \left(ns^{n-1}+(n-1)a_{n-1}s^{n-2}+\ldots+ a_1\right)\left(s^{n}+a_{n-1}s^{n-1}+\ldots+ a_1 s + a_0\right) z_t\\
 & = 0.
\end{align*}
\end{proof}

% \subsection{From Continuous Skolem Problem to Policy Synthesis over CTMDPs}\label{subsec:skolem_ctmdp}

We now move to the main reduction and provide the proofs of propositions presented in Section~\ref{sec:skolem_ctmdp}.

\smallskip

\begin{proof}[Proof of Proposition~\ref{prop:reduc1}]
We can show inductively that for any $k\in\set{0,1,2,\ldots}$, $\set{\alpha_1,\alpha_2,\ldots,\alpha_n}$, and $[\beta_1,\beta_2,\ldots, \beta_n]:= [\alpha_1,\alpha_2,\ldots, \alpha_n] A^k$, we have
\begin{align*}
& [\alpha_1,-\alpha_1,\alpha_2,-\alpha_2,\ldots, \alpha_n,-\alpha_n] \phi_1(A)^k= [\beta_1,-\beta_1,\beta_2,-\beta_2,\ldots, \beta_n,-\beta_n].
\end{align*}
Substitute $[\alpha_1,\alpha_2,\ldots,\alpha_n]$ by $C$ and $[\beta_1,\beta_2,\ldots, \beta_n]= CA^k$ to get
\begin{align*}
& C'' \phi_1(A)^k Y_2 = C''\phi_1(A)^k \phi_2(X_0) = [\beta_1,-\beta_1,\beta_2,-\beta_2,\ldots, \beta_n,-\beta_n] \phi_2(X_0)\\
& = [\beta_1,\beta_2,\ldots, \beta_n]X_0 = C A^k X_0\\
& \Rightarrow C'' e^{\phi_1(A)t}Y_2  = \sum_{k=0}^\infty \frac{t^k}{k!}C''\phi_1(A)^kY_2 = \sum_{k=0}^\infty \frac{t^k}{k!}C A^k X_0 = C e^{At} X_0.
\end{align*}
\end{proof}

\begin{comment}
Next, we define
\begin{equation*}
\lambda:=\max_i\sum_{j=1}^n|A_{ij}|+1,\quad P_2 := \phi_1(A)-\lambda \mathbb I_n,
\end{equation*}
and the vector $\mathbf{\beta}\in\mathbb Q^{2n}$ with
\begin{equation*}
\label{app:eq:beta}
\beta(2i-1)=\beta(2i)=\max (0,-P_2Y_2(2i-1),-P_2Y_2(2i))\quad 1\leq i \leq n
\end{equation*}
Note that the row sum of $P_2$ is at most $-1$ and $\beta+P_2Y_2$ is element-wise non-negative with the maximum element
\begin{equation*}
\label{app:eq:gamma}
\gamma:=\max_i P_2Y_2(i) + \beta(i).
\end{equation*}
\begin{proposition}
The above choices of $\lambda,\gamma$ and the matrix 
\begin{equation*}
\label{app:eq:P4}
P:=
\begin{bmatrix}
P_2 & \vdots & (P_2Y_2+\beta)/\gamma\\
\dots & \dots & \dots \\
\mathbf{0} &\vdots & 0
\end{bmatrix}
\end{equation*}
satisfy \eqref{app:eq:make_CTMDP} in Thm.~\ref{app:thm:existP}. Moreover, $P$ is row sub-stochastic.
\end{proposition}
\end{comment}

\begin{proof}[Proof of Proposition~\ref{prop:reduc2}]
We can easily show by induction that
\begin{equation*}
%\label{app:eq:P3_power}
P^k Y_0=\begin{bmatrix}
P_{2}^{k-1}(P_2Y_2+\boldsymbol\beta)/\gamma\\
0
\end{bmatrix},
\quad\forall k\in\set{1,2,\ldots}.
\end{equation*}
\begin{equation*}
C'e^{Pt}Y_0 = \sum_{k=0}^\infty \frac{t^k}{k!}C'P^k Y_0 = C'Y_0 + C'' \sum_{k=1}^\infty \frac{t^k}{k!}P_{2}^{k-1}(P_2Y_2+\boldsymbol\beta)/\gamma, 
\end{equation*}
where $C'':= [1,-1,\mathbf 0_{2n-2}]$ is the same vector as $C'$ but the last element is eliminated.
\begin{align*}
C'e^{Pt}Y_0 =  C'Y_0 +   C''e^{P_2t}Y_2/\gamma - C''Y_2/\gamma + \sum_{k=1}^\infty \frac{t^k}{k!}C''P_{2}^{k-1}\boldsymbol\beta/\gamma.
\end{align*}
The term $C'Y_0$ is zero by simple multiplication of the two vectors. $C''Y_2 = C''\phi_2(X_0) = X_0(1)$, which is also assumed to be zero. Finally, we see by induction that for all $k\in\set{1,2,\ldots}$, the elements $(2i-1)$ and $2i$ of the matrix $P_{2}^{k-1}\boldsymbol\beta$ are equal due to the particular structure of $P_2$ and $\boldsymbol\beta$. Therefore, the last sum in the above is also zero and we get
 \begin{align*}
C'e^{Pt}Y_0 & = C''e^{P_2t}Y_2/\gamma = C''e^{\phi_1(A)t-\lambda\mathbb I t}\phi_2(X_0)/\gamma \\
& = C''e^{\phi_1(A)t}\phi_2(X_0) e^{-\lambda t}/\gamma = C e^{At X_0} e^{-\lambda t}/\gamma.
\end{align*}
To show that $P$ is a sub-stochastic matrix, we recall that $P_2Y_2+\boldsymbol\beta\ge 0$ with maximum element $\gamma$. Then
\begin{equation*}
P_2\times\mathbf 1_{2n} + (P_2Y_2+\boldsymbol\beta)/\gamma\le  \phi_1(A)\mathbf 1_{2n}-\lambda\mathbf 1_{2n}+\mathbf 1_{2n} =  \phi_1(A)\mathbf 1_{2n} - \max_i\sum_{j}|A_{ij}|\le 0.
\end{equation*}
\end{proof}

\begin{proof}[Proof of Proposition~\ref{prop:selection_r}]
We have $W_0^\pi = \bar Y_0$ and $\mathcal F_k(W_0^\pi) =  \arg\max_{\dv} [\Qb^{\dv}]^k \bar Y_0$. Then, we need to compare $[\Qb^a]^k \bar Y_0$ with $[\Qb^b]^k \bar Y_0$ for different values of $k$ and see which one gives the first highest value. These two are the same for $k=1$ and
$\mathcal F_1(W_0^\pi) =  \arg\max_{\dv} \Qb^{\dv} \bar Y_0 = \{\dv_a,\dv_b\}$.
Suppose For $k_0>1$ is the smallest index such that $\bar C[\Qb^a]^{k_0}\bar Y_0\neq 0$. It can be shown inductively that $[{\Qb^b}]^k \bar Y_0 = [{\Qb^a}]^k \bar Y_0$ for all $1\le k\le k_0$: 
\begin{align*}
[{\Qb^b}]^k \bar Y_0 & = {\Qb^b}[{\Qb^b}]^{k-1} \bar Y_0 = (\Qb^a+K)[{\Qb^b}]^{k-1} \bar Y_0 = (\Qb^a+K)[{\Qb^a}]^{k-1} \bar Y_0 \\
& = [{\Qb^a}]^k \bar Y_0 + K[{\Qb^a}]^{k-1} \bar Y_0= 
[{\Qb^a}]^k \bar Y_0 - r \begin{bmatrix}
\bar C [{\Qb^a}]^{k-1} \bar Y_0 \\
\mathbf 0_{(2n+1)\times 2n}
\end{bmatrix}
 = [{\Qb^a}]^k \bar Y_0.
\end{align*}
This means $\mathcal F_k(W_0^\pi) =  \arg\max_{\dv} [\Qb^{\dv}]^k \bar Y_0 = \{\dv_a,\dv_b\}$ for all $1\le k\le k_0$. We have for $k=k_0+1$
\begin{align*}
[{\Qb^b}]^{k_0+1} \bar Y_0 & =
[{\Qb^a}]^{k_0+1} \bar Y_0 - r \begin{bmatrix}
\bar C [{\Qb^a}]^{k_0} \bar Y_0 \\
\mathbf 0_{(2n+1)\times 2n}.
\end{bmatrix}
\end{align*}
The first element of $[{\Qb^b}]^{k_0+1} \bar Y_0$ is strictly less than the first element of $[{\Qb^a}]^{k_0+1} \bar Y_0$ since $r$ has the same sign as $\bar C [{\Qb^a}]^{k_0} \bar Y_0$. Thus $\mathcal F_{k_0+1}(W_0^\pi) =  \arg\max_{\dv} [\Qb^{\dv}]^{k_0+1} \bar Y_0 = \{\dv_a\}$.
\end{proof}
